# Supplementary material for: Reinforcement Learning of POMDPs using Spectral Methods
Source: arXiv:1602.07764 source file (2016-05-29)
Supplement: Supplementary file 1 [file table_appendix.tex]

% !TEX root = master.tex
